# Supplementary material for: Charge Transfer as a Ubiquitous Mechanism in Determining the Negative Charge at Hydrophobic Interfaces
Source: arXiv:1904.05766 ancillary file (2019-04-12)
Supplement: Supplementary file 1 [file Supporting_info.pdf]

# Charge Transfer as a Ubiquitous Mechanism in Determining the Negative Charge at Hydrophobic Interfaces

# Supporting Information

Emiliano Poli,* Kwang H. Jong, and Ali Hassanali*

*Condensed Matter Statistical Physics Department, The Abdus Salam International Center for Theoretical Physics, Strada Costiera, Trieste*

E-mail: epoli@ictp.it; ahassanali@ictp.it

## The Air/Oil Water Interfaces are Negatively Charged

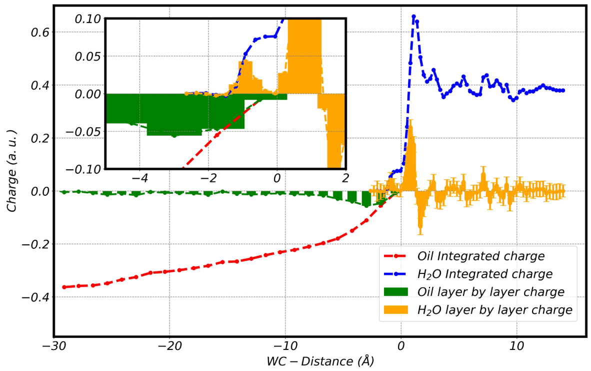


Figure 1: Charge (yellow bars) and integrated surface charge (blue line) obtained for the DDEC charges extracted from our calculations for the water-oil interface. For the oil phase the charge is reported using green bars and the integrated surface charge is shown by red line. The inset magnifies the charge oscillations right at the interface between the two phases.

## Charging is Coupled to the Local Topology and Environment

| Water-air | | | | |
|---|---|---|---|---|
| **2in-1out** | **2in-2out** | **1in-2out** | **1in-1out** | **1in-0out** |
| 0.02258 | | -0.02074 | -0.00163 | 0.03183 |
| 0.02933 | -0.00279 | -0.02836 | -0.00049 | 0.02728 |
| 0.02419 | 0.00270 | -0.02291 | -0.00020 | 0.02555 |
| 0.02146 | 0.00262 | -0.02249 | -0.00085 | 0.02024 |
| **Water-oil** | | | | |
| **2in-1out** | **2in-2out** | **1in-2out** | **1in-1out** | **1in-0out** |
| 0.02522 | 0.00613 | -0.01465 | 0.00144 | 0.03077 |
| 0.02583 | 0.00235 | -0.02223 | 0.00187 | 0.02603 |
| 0.02320 | 0.00205 | -0.02337 | -0.00202 | 0.02184 |
| 0.02197 | 0.00240 | -0.02209 | -0.00235 | 0.02152 |

Figure 2: First moment of the layer-by-layer charge distributions for the different water molecules coordination types. The upper table values refers to Figure 4 in the main text, the lower one to Figure 6. Where values are not present it was not possible to calculate a reliable distribution due to small population.

## Electronic characterization of the water-air, oil-water interfaces

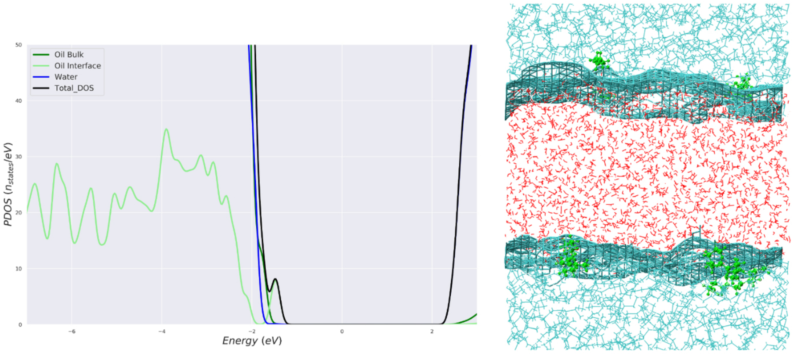


Figure 3: Representation of the water-oil interface edge of the valence band (EVB) electronic structure. The LDOS in the left panel is obtained considering the states belonging to the oil molecules at the interface (distance from the WCI < 5.0 Å) in the bulk and to water phase. This frame is characteristic of the fluctuations where the EVB is mainly comprised by states belonging to the negatively charged oil. The right panel highlights the molecules that characterize the EVB.

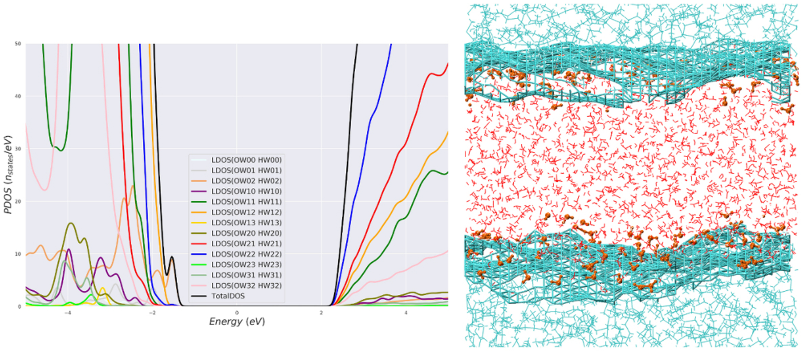


Figure 4: Representation of the water-oil interface edge of the valence band (EVB) electronic structure. The LDOS in the left panel is obtained considering the states belonging to the different types of water coordination species. This frame is characteristic of the fluctuations where the EVB is mainly comprised by states belonging to the water phase. The right panel highlights the molecules that characterize the EVB.

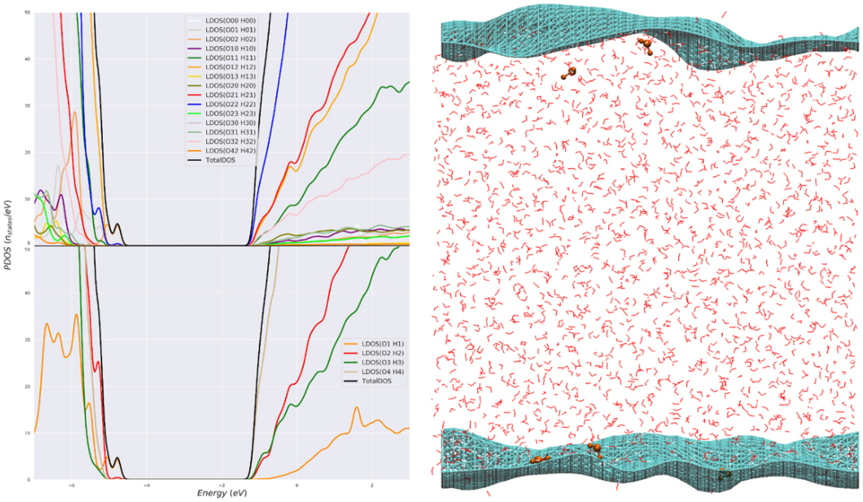


Figure 5: Sample representation of the water-air interface edge of the valence band (EVB) electronic structure. The Local Density of States (LDOS) in the top-left panel is obtained by projecting the states for the different water coordination species. The one in the bottom-left Panel is obtained considering the projection for the water molecules belonging to the different layers defined starting from the Willard Chandler Interface (WCI) and moving towards the bulk. The water molecules belonging to the EVB in both these projections are highlighted in orange in the right panel.
